# Supplementary material for: Privacy Leakage of Adversarial Training Models in Federated Learning Systems
Source: arXiv:2202.10546 source file (2022-02-21)
Supplement: Supplementary file 1 [file appendix.tex]

\appendix
\onecolumn

\begin{center}
\Large
\textbf{Appendix}
\end{center}
